# Supplementary material for: TESTNAV: Pareto-Guided Search for Compositional Robustness Testing
Source: arXiv:2608.19882 source file (2026-08-20)
Supplement: Supplementary file 1 [file appendix_pareto_auto.tex]

% ==============================================
% Auto-generated appendix
% ==============================================
\newcommand{\pimg}[1]{%
  \includegraphics[width=0.13\linewidth]{#1}
}

\subsection{SSIM Family ($|\mathcal{P}^*| = 27$)}
\label{app:pareto:ssim}

\subsubsection*{$\Theta_1$: 9 configurations}
\begin{figure}[p]
\centering
\pimg{pareto_examples/ssim_chrf/order1/01_P1-0_P2-5_P3-0_P4-0}%
\pimg{pareto_examples/ssim_chrf/order1/02_P1-0_P2-4_P3-0_P4-0}%
\pimg{pareto_examples/ssim_chrf/order1/03_P1-0_P2-0_P3-0_P4-5}%
\pimg{pareto_examples/ssim_chrf/order1/04_P1-0_P2-0_P3-0_P4-4}%
\pimg{pareto_examples/ssim_chrf/order1/05_P1-0_P2-2_P3-0_P4-0}%
\pimg{pareto_examples/ssim_chrf/order1/06_P1-0_P2-0_P3-0_P4-3}%
\pimg{pareto_examples/ssim_chrf/order1/07_P1-0_P2-0_P3-0_P4-2}%
\pimg{pareto_examples/ssim_chrf/order1/08_P1-0_P2-0_P3-0_P4-1}%
\pimg{pareto_examples/ssim_chrf/order1/09_P1-0_P2-0_P3-0_P4-0}%
\caption{ImageNet ($\mathcal{P}^*$, SSIM) --- $\Theta_1$: 9 Pareto configs with 1 active perturbation. Each combination $(P_1,P_2,P_3,P_4)$ is annotated with $\updelta$ and $\uprho$.
}
\label{fig:app:ssim:order1}
\end{figure}

\subsubsection*{$\Theta_2$: 12 configurations}
\begin{figure}[p]
\centering
\pimg{pareto_examples/ssim_chrf/order2/01_P1-4_P2-5_P3-0_P4-0}%
\pimg{pareto_examples/ssim_chrf/order2/02_P1-3_P2-5_P3-0_P4-0}%
\pimg{pareto_examples/ssim_chrf/order2/03_P1-2_P2-5_P3-0_P4-0}%
\pimg{pareto_examples/ssim_chrf/order2/04_P1-1_P2-5_P3-0_P4-0}%
\pimg{pareto_examples/ssim_chrf/order2/05_P1-2_P2-4_P3-0_P4-0}%
\pimg{pareto_examples/ssim_chrf/order2/06_P1-1_P2-4_P3-0_P4-0}%
\pimg{pareto_examples/ssim_chrf/order2/07_P1-0_P2-2_P3-0_P4-5}%
\pimg{pareto_examples/ssim_chrf/order2/08_P1-1_P2-0_P3-0_P4-5}%
\pimg{pareto_examples/ssim_chrf/order2/09_P1-0_P2-0_P3-1_P4-5}%
\pimg{pareto_examples/ssim_chrf/order2/10_P1-0_P2-0_P3-1_P4-4}%
\pimg{pareto_examples/ssim_chrf/order2/11_P1-1_P2-2_P3-0_P4-0}%
\pimg{pareto_examples/ssim_chrf/order2/12_P1-0_P2-0_P3-1_P4-3}%
\caption{ImageNet ($\mathcal{P}^*$, SSIM) --- $\Theta_2$: 12 Pareto configs with 2 active perturbations. Each combination $(P_1,P_2,P_3,P_4)$ is annotated with $\updelta$ and $\uprho$.
}
\label{fig:app:ssim:order2}
\end{figure}

\subsubsection*{$\Theta_3$: 4 configurations}
\begin{figure}[p]
\centering
\pimg{pareto_examples/ssim_chrf/order3/01_P1-1_P2-5_P3-1_P4-0}%
\pimg{pareto_examples/ssim_chrf/order3/02_P1-2_P2-2_P3-0_P4-5}%
\pimg{pareto_examples/ssim_chrf/order3/03_P1-1_P2-2_P3-0_P4-5}%
\pimg{pareto_examples/ssim_chrf/order3/04_P1-1_P2-2_P3-0_P4-4}%
\caption{ImageNet ($\mathcal{P}^*$, SSIM) --- $\Theta_3$: 4 Pareto configs with 3 active perturbations. Each combination $(P_1,P_2,P_3,P_4)$ is annotated with $\updelta$ and $\uprho$.
}
\label{fig:app:ssim:order3}
\end{figure}

\subsubsection*{$\Theta_4$: 2 configurations}
\begin{figure}[p]
\centering
\pimg{pareto_examples/ssim_chrf/order4/01_P1-1_P2-5_P3-1_P4-1}%
\pimg{pareto_examples/ssim_chrf/order4/02_P1-2_P2-2_P3-1_P4-5}%
\caption{ImageNet ($\mathcal{P}^*$, SSIM) --- $\Theta_4$: 2 Pareto configs with 4 active perturbations. Each combination $(P_1,P_2,P_3,P_4)$ is annotated with $\updelta$ and $\uprho$.
}
\label{fig:app:ssim:order4}
\end{figure}

\subsection{KID Family ($|\mathcal{P}^*| = 27$)}
\label{app:pareto:kid}

\subsubsection*{$\Theta_1$: 4 configurations}
\begin{figure}[p]
\centering
\pimg{pareto_examples/kid_bert/order1/01_P1-0_P2-0_P3-0_P4-2}%
\pimg{pareto_examples/kid_bert/order1/02_P1-0_P2-0_P3-2_P4-0}%
\pimg{pareto_examples/kid_bert/order1/03_P1-0_P2-0_P3-1_P4-0}%
\pimg{pareto_examples/kid_bert/order1/04_P1-0_P2-0_P3-0_P4-0}%
\caption{ImageNet ($\mathcal{P}^*$, KID) --- $\Theta_1$: 4 Pareto configs with 1 active perturbation. Each combination $(P_1,P_2,P_3,P_4)$ is annotated with $\updelta$ and $\uprho$.
}
\label{fig:app:kid:order1}
\end{figure}

\subsubsection*{$\Theta_2$: 7 configurations}
\begin{figure}[p]
\centering
\pimg{pareto_examples/kid_bert/order2/01_P1-0_P2-0_P3-4_P4-2}%
\pimg{pareto_examples/kid_bert/order2/02_P1-2_P2-0_P3-0_P4-2}%
\pimg{pareto_examples/kid_bert/order2/03_P1-0_P2-0_P3-3_P4-2}%
\pimg{pareto_examples/kid_bert/order2/04_P1-0_P2-2_P3-0_P4-2}%
\pimg{pareto_examples/kid_bert/order2/05_P1-0_P2-0_P3-2_P4-2}%
\pimg{pareto_examples/kid_bert/order2/06_P1-0_P2-1_P3-0_P4-2}%
\pimg{pareto_examples/kid_bert/order2/07_P1-0_P2-0_P3-1_P4-2}%
\caption{ImageNet ($\mathcal{P}^*$, KID) --- $\Theta_2$: 7 Pareto configs with 2 active perturbations. Each combination $(P_1,P_2,P_3,P_4)$ is annotated with $\updelta$ and $\uprho$.
}
\label{fig:app:kid:order2}
\end{figure}

\subsubsection*{$\Theta_3$: 14 configurations}
\begin{figure}[p]
\centering
\pimg{pareto_examples/kid_bert/order3/01_P1-0_P2-5_P3-3_P4-2}%
\pimg{pareto_examples/kid_bert/order3/02_P1-0_P2-5_P3-2_P4-2}%
\pimg{pareto_examples/kid_bert/order3/03_P1-0_P2-5_P3-1_P4-2}%
\pimg{pareto_examples/kid_bert/order3/04_P1-1_P2-0_P3-5_P4-2}%
\pimg{pareto_examples/kid_bert/order3/05_P1-3_P2-0_P3-3_P4-2}%
\pimg{pareto_examples/kid_bert/order3/06_P1-2_P2-0_P3-4_P4-2}%
\pimg{pareto_examples/kid_bert/order3/07_P1-1_P2-0_P3-4_P4-2}%
\pimg{pareto_examples/kid_bert/order3/08_P1-2_P2-0_P3-3_P4-2}%
\pimg{pareto_examples/kid_bert/order3/09_P1-0_P2-1_P3-4_P4-2}%
\pimg{pareto_examples/kid_bert/order3/10_P1-1_P2-0_P3-3_P4-2}%
\pimg{pareto_examples/kid_bert/order3/11_P1-1_P2-0_P3-2_P4-2}%
\pimg{pareto_examples/kid_bert/order3/12_P1-0_P2-1_P3-3_P4-2}%
\pimg{pareto_examples/kid_bert/order3/13_P1-0_P2-2_P3-2_P4-2}%
\pimg{pareto_examples/kid_bert/order3/14_P1-0_P2-1_P3-2_P4-2}%
\caption{ImageNet ($\mathcal{P}^*$, KID) --- $\Theta_3$: 14 Pareto configs with 3 active perturbations. Each combination $(P_1,P_2,P_3,P_4)$ is annotated with $\updelta$ and $\uprho$.
}
\label{fig:app:kid:order3}
\end{figure}

\subsubsection*{$\Theta_4$: 2 configurations}
\begin{figure}[p]
\centering
\pimg{pareto_examples/kid_bert/order4/01_P1-1_P2-5_P3-1_P4-1}%
\pimg{pareto_examples/kid_bert/order4/02_P1-1_P2-5_P3-1_P4-2}%
\caption{ImageNet ($\mathcal{P}^*$, KID) --- $\Theta_4$: 2 Pareto configs with 4 active perturbations. Each combination $(P_1,P_2,P_3,P_4)$ is annotated with $\updelta$ and $\uprho$.
}
\label{fig:app:kid:order4}
\end{figure}
